# Supplementary material for: Charging-driven coarsening and melting of a colloidal nanoparticle monolayer at an ionic liquid-vacuum interface
Source: arXiv:2008.00652 ancillary file (2020-09-08)
Supplement: Supplementary file 1 [file ESI.pdf]

# Electronic Supplementary Information For

## Charging-driven coarsening and melting of a colloidal nanoparticle monolayer at an ionic liquid-vacuum interface

Connor G. Bischak, Jonathan G. Raybin, Jonathon W. Kruppe, and Naomi S. Ginsberg

E-mail: nsginsberg@berkeley.edu

This PDF file includes:
Lindemann Criterion, Simulations, and Modeling
Supplementary Figures and Tables
Supplementary Movie Caption
Supplementary References

## Lindemann criterion, Simulations, and Modeling

### Lindemann Criterion

Here, we summarize the procedure we used to establish a Lindemann criterion. The Lindemann criterion is widely used to characterize melting transitions. It states that melting occurs when the fluctuations of lattice points become large compared to lattice spacings. The Lindemann parameter used for three-dimensional systems, however, is proportional to the particle mean squared displacements and diverges for 2D systems in the crystal and liquid phase [1–5]. A Lindemann-like criterion has been developed [1, 2] and used to quantify melting transitions in 2D colloidal systems [2–6]. This 2D Lindemann-like criterion is assessed for the dynamic (2D) Lindemann parameter, described here as a single particle variation that otherwise follows the treatment in Kelleher et al.[6]:

$$LP_j(\tau) = \frac{\langle(\frac{1}{N_{nn}}\sum_k^{N_{nn}} \Delta r_j(\tau,t) - \Delta r_k(\tau,t))^2\rangle}{2a^2} \tag{S1}$$

where $\Delta r_j(\tau,t) = r_j(\tau+t) - r_j(t)$ is the displacement vector of particle $j$ from time t to time t + $\tau$, $a$ is the lattice spacing, $N_{nn}$ is the number of nearest neighbors to particle $j$ at a time $t$. To relate to a criterion for melting, this single particle Lindemann parameter is averaged over all particles $j$ to obtain information about the phase of the ensemble. The averaging over $t$ is carried out as follows: the argument of the average is calculated throughout the entire experiment in time intervals of fixed duration $\tau$ for each time point $t$. The value of this Lindemann parameter for a given $\tau$ is then the average of this argument, taken over all of the time intervals, which share a common duration $\tau$ and differ by their starting time $t$.

In Kelleher et al.,[6] the phase of the system was determined by the behavior of the Lindemann parameter averaged over all particles $j$, $LP(\tau)$, at a fixed system temperature, as $\tau$ is increased. For a solid, the system Lindemann parameter remains constant as the time interval $\tau$ grows large, whereas for a liquid, the system Lindemann parameter should diverge. This behavior can be rationalized by noting that in the liquid phase, we expect the motion of particles at time $t+\tau$ to be uncorrelated with that of their nearest neighbors from time $t$ for long $\tau$. By studying the behavior of $LP(\tau)$ in the long $\tau$ limit at various temperatures, one can identify the temperature at which the melting transition occurs. The transition temperature will be approximately given by the first temperature at which the Lindemann parameter diverges at long $\tau$.

Rather than induce a melting transition by increasing the temperature, we fix the temperature and decrease the area fraction by driving the system with the electron beam. Due to the perturbative nature of this measurement, we do not maintain a constant area fraction for consecutive frames, and cannot apply the Lindemann criterion in the form described above. We thus perform a modified Lindemann criterion analysis, which is based on the procedure described above. We calculate $LP_j(\tau_0,t)$ the instantaneous Lindemann parameter for each frame $t$ for each particle $j$ with a fixed value of $\tau$ = $\tau_0$ of 2.56 s, the time between frames. This instantaneous single particle Lindemann parameter can then be averaged over all particles $j$ in the ensemble (as is customarily done) to obtain:

$$LP(\tau_0,t) = \langle LP_j(\tau_0,t)\rangle_j = \langle\frac{((\frac{1}{N_{nn}}\sum_k^{N_{nn}} \Delta r_k(\tau_0,t))^2}{2a^2}\rangle_j \tag{S2}$$

Note that the time average has been removed, as compared with Equation S1. Whereas $LP_j(\tau_0,t)$ is used to false color the individual particles in Figures 3B and 4A, the average Lindemann parameter for all particles in the monolayer at a given time in Equation S2 is presented in the plots in Figures 4D and S8B. Both are calculated using the displacement vectors for each particle $j$ of $\Delta r_j(\tau_0,t) = r_j(\tau_0+t) - r_j(t)$. By employing a fixed value of $\tau$ equal to the frame duration, and by eliminating the time average, we are able to capture an instantaneous representation of the Lindemann parameter at a fixed area fraction, and we repeat the evaluation as a function of time, and hence, as a function of area fraction. We expect that this 2.56 s period, throughout which the electron beam raster scans the sample, is large enough for the particles to explore their local configuration space, and thus gives a strong estimate of the phase of the system. We therefore take our frame-to-frame values of the Lindemann parameter to each operate in the aforementioned 'long $\tau$ limit'. By displaying this frame-to-frame system Lindemann parameter vs time, as we do in Figures 4D

and S8B, we are able to identify the temporal onset of the melting transition as the time at which our system Lindemann parameter begins to rapidly increase and cross the threshold value of 0.04.

### Lennard-Jones model suitability

To further investigate the nature of the interparticle interactions, we performed simulations using the Weeks-Chandler-Anderson (WCA) potential [7] to approximate hard-sphere interactions in LAMMPS. The WCA potential is given by:

$$u(r_{ij}) = \begin{cases} 4\epsilon[(\frac{\sigma}{r_{ij}})^{12} - (\frac{\sigma}{r_{ij}})^{6}] + \epsilon & r \leq 2^{1/6}\sigma \\ 0 & r > 2^{1/6}\sigma \end{cases} \quad \text{(S3)}$$

The results of the WCA simulation are given in Figure S8, with the same analysis parameters as shown in Figure 4C-F of the main text. For comparison, the results of the Lennard-Jones simulations, as well as the experimental data are shown together. Both simulations in Figure S8 were conducted at a reduced temperature of $T = 0.75$. The WCA simulations display a faster phase dynamics, exhibiting qualitative disagreement with experiment in comparison to the Lennard-Jones model. This late time period corresponds to a semi-dilute regime, where the 2D system has undergone a melting transition. We also performed WCA simulations across a range of different temperatures, and found that the disagreement between WCA and experiment persists. That the attractive portion of the Lennard-Jones potential is necessary to recapitulate the experimental results suggests attractive interactions are present in our system.

### Unpinning Model

Colloidal particles initially assemble at the IL/vacuum interface to minimize interfacial energy, as shown in Figure S7A. The free energy contribution of interfacial pinning is determined from the balance of interactions between the particle, liquid, and vacuum phases. Using Young's equation,

$$\cos\theta = \frac{\gamma_{S-V} - \gamma_{S-L}}{\gamma_{L-V}}, \quad \text{(S4)}$$

the pinning energy of a particle with radius $r$ can be expressed in terms of the contact angle $\theta$ and the IL/vacuum surface tension $\gamma_{L-V}$:

$$\Delta E = \pi r^2 \gamma_{L-V}(1 - \cos\theta)^2. \quad \text{(S5)}$$

Figure S7B shows the interfacial pinning energy of an individual nanoparticle as a function of contact angle. Calculations are performed using literature and reference parameters collected in Table S1. For 300-nm-diameter particles, we calculate substantial pinning energies greater than 1000 $k_B T$ for initial contact angles of $\theta \sim 20°$. Thermal desorption of particles from the interface is not expected until the contact angle decreases below roughly 2°, at which point pinning energies are on the order of several $k_B T$.

As particles charge, the IL reorganizes around the particles to form a capacitive double-layer. Dielectric screening by the IL increases the particle wetting affinity which lowers the contact angle. This electrowetting behavior as a function of the surface potential $\psi$ is described by the Young-Lippmann equation:[8, 9]

$$\Delta\cos\theta = \frac{\epsilon_0 \epsilon_r}{\lambda_D \gamma_{L-V}} \frac{(2k_B T)^2}{e^2}(\cosh(\frac{e\psi}{k_B T}) - 1). \quad \text{(S6)}$$

Here, $\epsilon_0$ and $\epsilon_r$ are the vacuum permittivity constant and the IL dielectric constant, respectively, $\lambda_D$ is the IL Debye length, and $e$ is the electron charge. There is uncertainty in the particular choice of Debye length. We select a value of 3 Å to reflect the capacative screening length scale of the double-layer.[10–12] Shown in Figure S7C, this expression describes changes in surface wetting as a function of surface potential by accounting for the influence of the IL surface tension and capacitive screening. By parameterizing the contact angle, we can directly assess how the particle pinning energy varies during charging. The results of this combined analysis, shown in Figure S7D, indicate a sharp decrease in pinning energy at around 70 mV. Above this value, particles detach from the interface and dissolve into the bulk IL droplet. Although the shape of the curve is striking, the specific threshold is reliant on many reference parameters. Still, we expect that unpinning occurs at surface potentials of order 10-100 mV.

### Modeling of accelerating voltage dependence

Monte Carlo modeling of electron beam scattering, shown in Figure S9A, measures how energy is deposited with varying beam voltages. At 2 kV, energy is preferentially deposited near the particle surface and becomes more uniformly distributed as the beam energy is increased. Although not captured in this model, we expect the particles to freely rotate on experimental time scales, leading to spherically symmetric distributions. The overall sign of charging is determined by whether there is net scattering of secondary electrons or net implantation of primary electrons, and this balance is dependent on the beam's accelerating voltage (Figure S9B). From Monte Carlo simulations, we find net negative charging in this voltage regime. As the accelerating voltage is increased, we measure a greater than 90% decrease in the fraction of trapped primary electrons alongside a roughly 50% decrease in the secondary electron yield. This large decrease in primary electron trapping occurs because the size of the interaction volume expands to include the entire particle, increasing the fraction of transmitted and backscattered electrons that escape the particle. Meanwhile, secondary electrons are predominantly emitted from near the surface and are less impacted by the size of the interaction volume. Consequently, the net charge balance becomes less negative and smaller in magnitude with increasing accelerating voltage. Altogether, the surface potential increases more slowly at higher beam voltages, which in turn leads to the later observed unpinning times.

Based on this model, we predict that each particle will detach from the interface once its total charge yields a surface potential above this threshold. The observed particle fraction, plotted in Figure S10, shows a distribution of unpinning times for each beam voltage. We fit these curves by modeling the particle fraction $\rho(t)$ as a cumulative distribution function with characteristic unpinning time $t_s$ and a time-dependent standard deviation $\sigma(t)$:

$$\rho(t) = \frac{1}{2}(1 - \mathrm{erf}(\frac{t - t_s}{\sqrt{2}\sigma(t)}))\ ;\ \sigma(t) = kt \tag{S7}$$

The average unpinning time is beam voltage-dependent, due to differences in the electron transmission rate, as discussed above. Fit parameters are collected in Table S2. This model is consistent with a system of normally distributed particle charges in which the standard deviation increases linearly over the experimental time, suggesting that variability in unpinning time results from heterogeneities in the charging rate. For each voltage, we find $k \sim 0.3\ \mathrm{s}^{-1}$. Differences in charging rate are dependent on the local particle environment as well as the effective electron dose across the imaging field of view. We note that variation due to thermal fluctuations or beam current shot noise are negligible compared to the observed unpinning distributions.

## Supplementary Figures and Tables

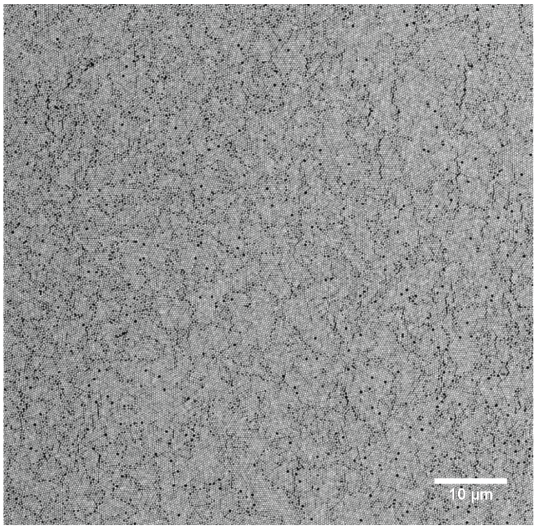


**Fig. S1.** Large field of view of a colloidal monolayer self-assembled at the interface between the IL and vacuum.

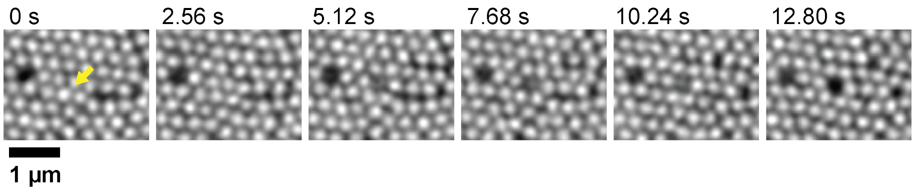


**Fig. S2.** Time series of SE images showing a single colloidal particle disappearing over time (indicated by the yellow arrow in the first frame).

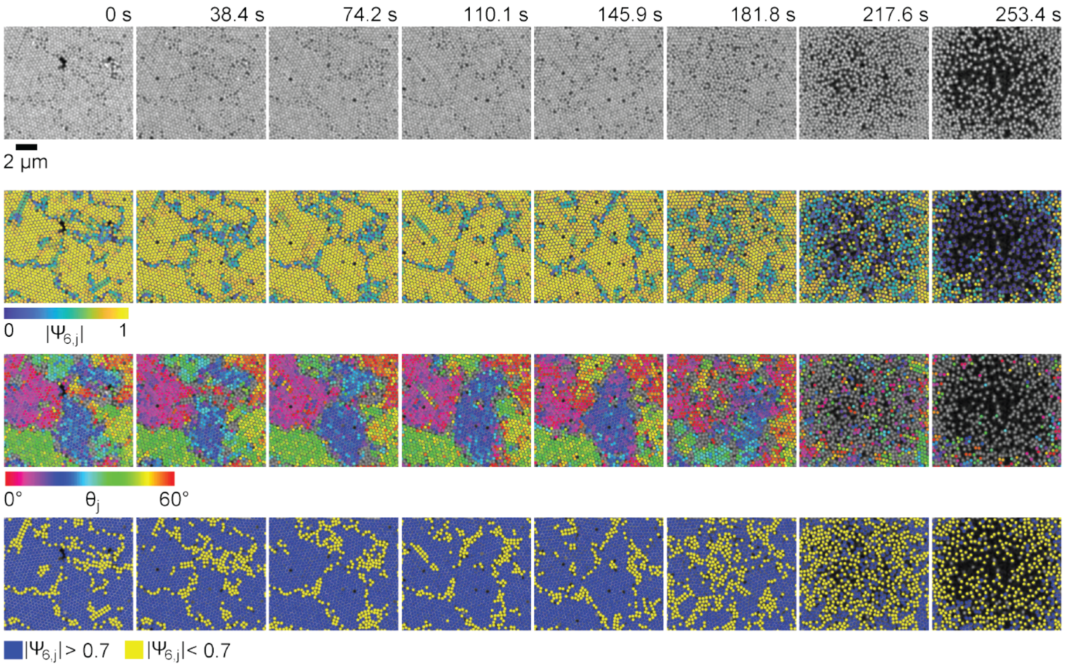


**Fig. S3.** An additional dataset acquired under the same conditions as those described in the main text.

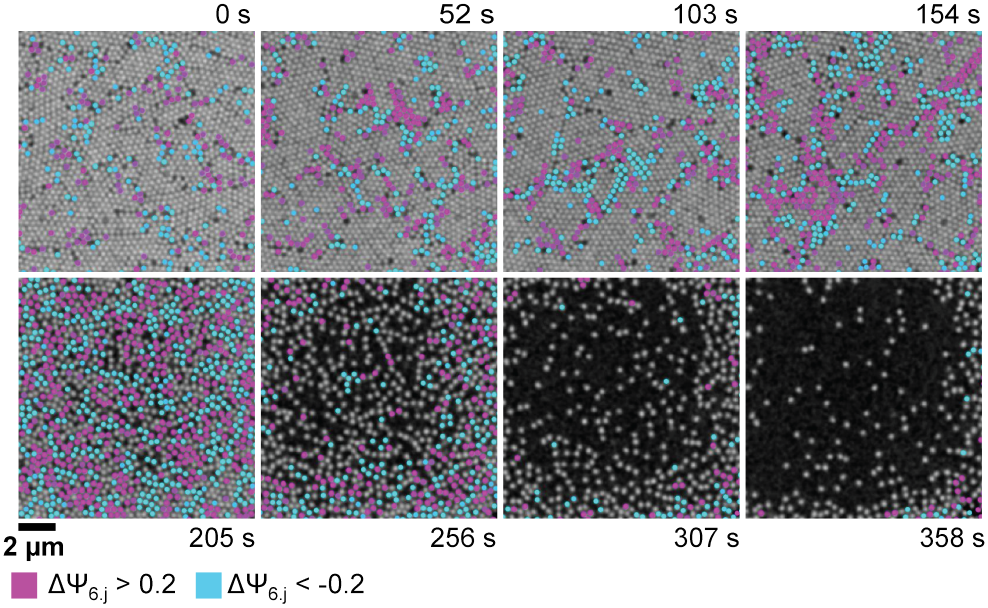


**Fig. S4.** Frame-to-frame fluctuations in local crystallinity indicated by the frame-to-frame change in the bond order parameter ($\Delta|\Psi_{6,j}|$). Particles becoming more ordered are magenta ($\Delta|\Psi_{6,j}| > 0.2$) and particles becoming less crystalline are cyan ($\Delta|\Psi_{6,j}| < 0.2$).

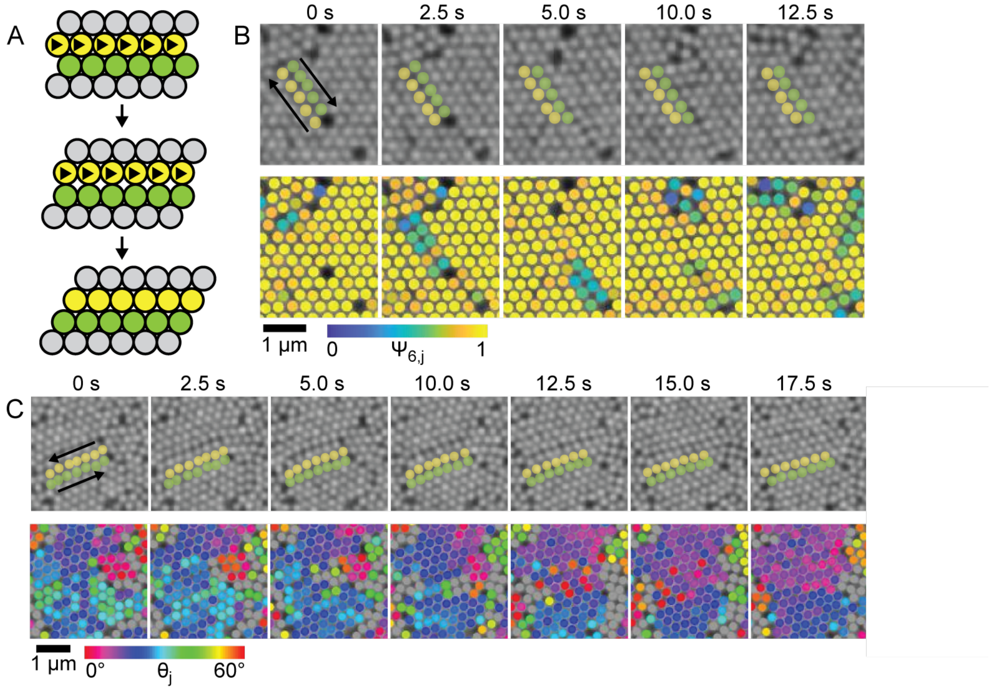


**Fig. S5.** Sliding dislocations underlie many dynamical changes at larger scales. (A) Schematic of a sliding dislocation. (B) Time series of SE images showing an example of a sliding dislocation transporting a point vacancy to a more disordered region with the corresponding images false colored by $|\Psi_{6,j}|$. (C) Time series of SE images showing an example of a sliding dislocation reorienting a crystalline domain with the corresponding images false colored based on $\theta_j$.

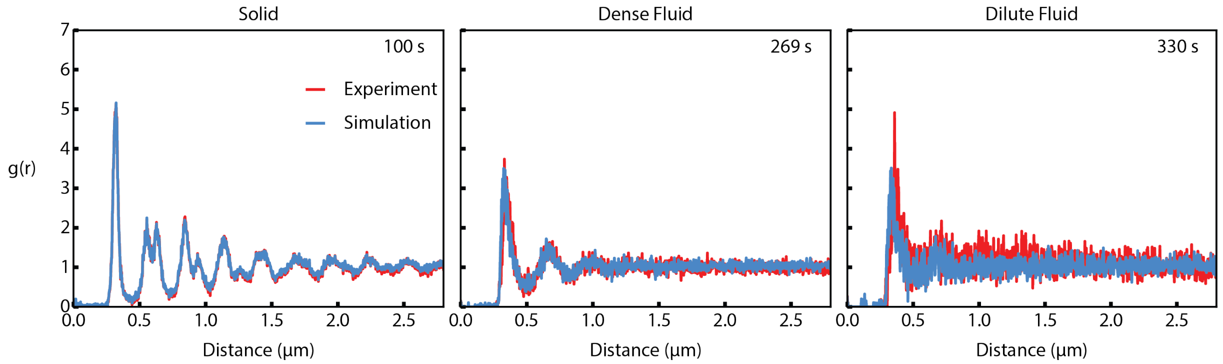


**Fig. S6.** The radial distribution function, $g(r)$, shows agreement between experiment and simulation. The $g(r)$ is shown for the experimental data and the Lennard-Jones model, in the (A) solid phase at 100 s, (B) dense fluid phase at 269 s, and (C) dilute fluid phase at 330 s. Both experimental and numerical data display ordering of a hexagonal lattice in the crystalline phase at 100 s. As particles are removed from the system, both simulation and experiment exhibit a similar breakdown of translational order, as a fluid phase emerges on similar time scales in both. This similarity indicates strong qualitative agreement between the Lennard-Jones model and the experimental data, in addition to that shown in Figure 4C-F in the main text.

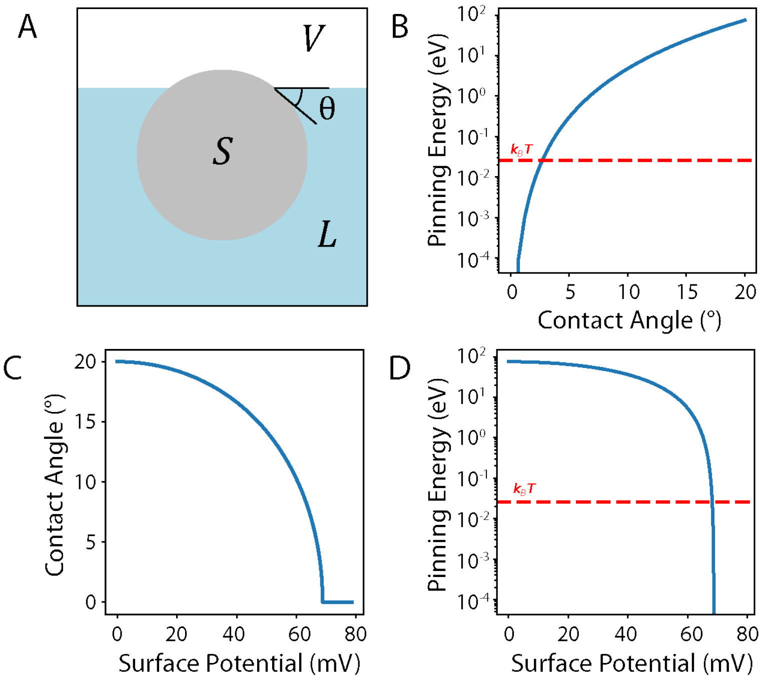


**Fig. S7.** Unpinning Model. (A) Contact angle of a particle at the vacuum/IL interface. (B) Log plot of interfacial pinning energy of a single particle as a function of contact angle. The pinning energy is much greater than $k_B T$ (red dashed line) for contact angles above $\sim 3°$. (C) Plot of contact angle as a function of surface potential, based on the Young-Lippmann equation, Equation S6. (D) Log plot of pinning energy with increasing surface potential. The pinning energy becomes comparable to $k_B T$ at a surface potential of roughly 70 mV.

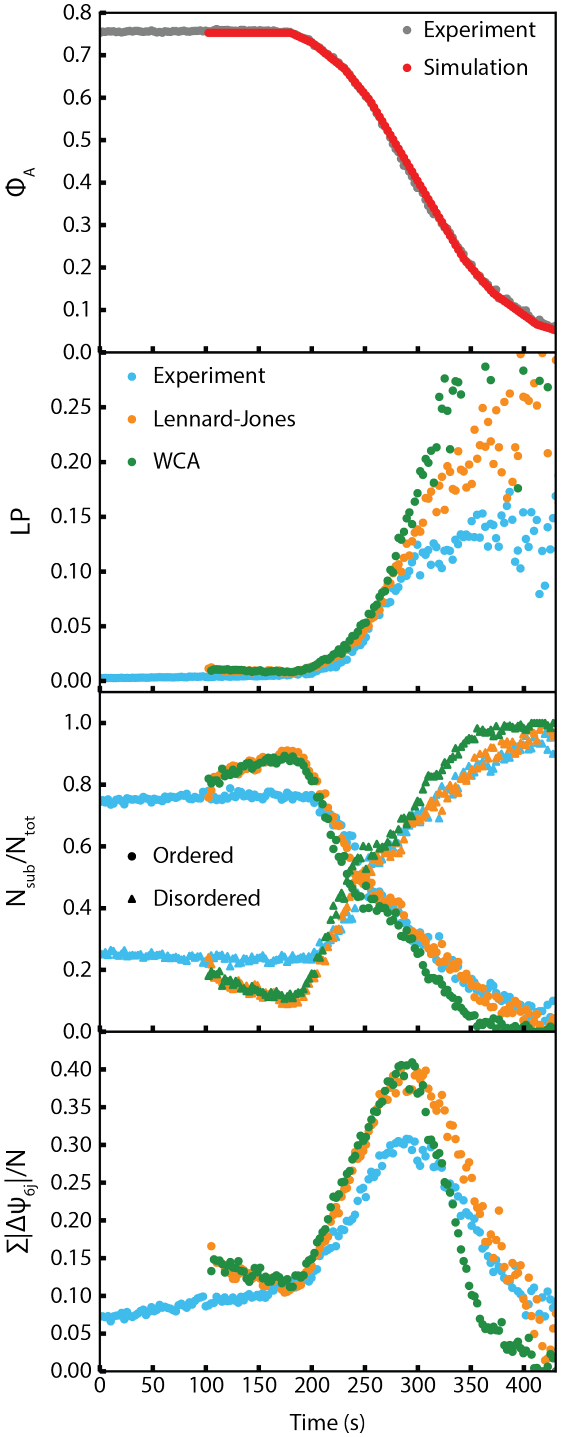


**Fig. S8.** Comparison of hard sphere and Lennard-Jones model. (A) The area fraction of the simulation is determined by closely matching the experimentally measured one and is kept the same amongst all simulation trials. (B) The Lindemann parameter for the WCA model qualitatively diverges faster than experiment, (inset) yet crosses the melting threshold at approximately the same time. The strong repulsion and lack of attraction in the WCA model drives the orientational order of the simulation ensemble to (C) coarsen on shorter time scales and (D) fluctuate more dramatically.

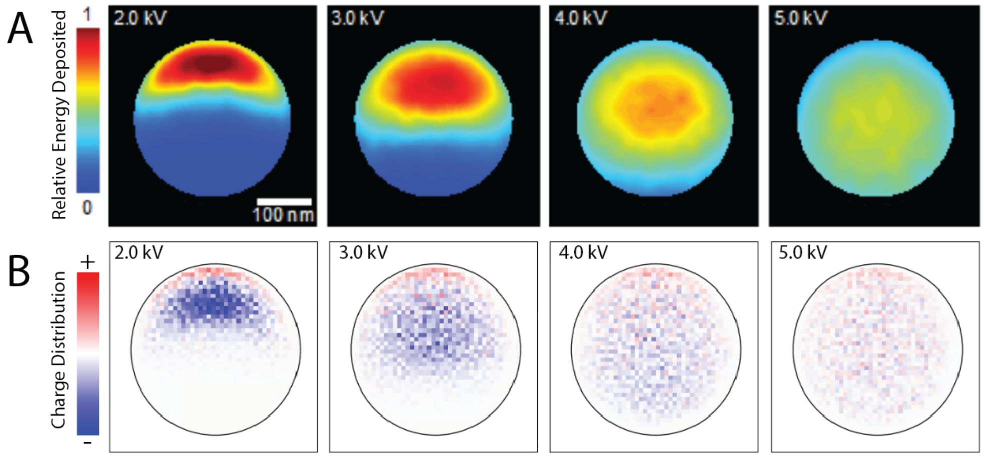


**Fig. S9.** (A) Simulated energy deposition of primarily electrons in a 300 nm silica sphere by electron beam as a function of accelerating voltage, as also shown in the main text Figure 6B. The same energy scale is employed for all four cases to facilitate direct comparison. (B) Simulated charge distributions as a function of accelerating voltage. Positive charging results from the scattering of secondary electrons, and negative charging is due to the trapping of primary electrons. The same charge scale is used for all four cases.

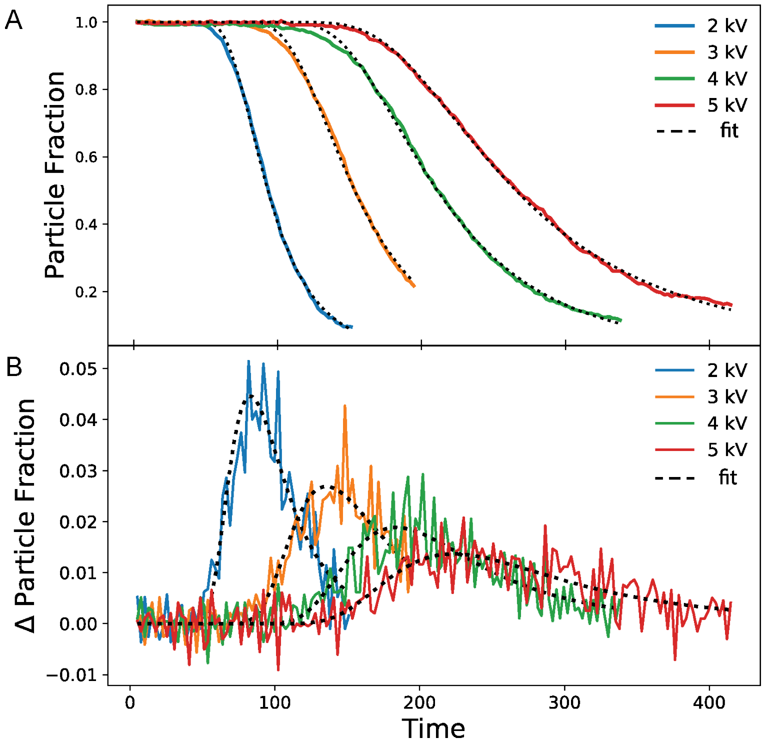


**Fig. S10.** (A) Plot of particle fraction as a function of time for 2-5 kV fit with Equation S7. (B) Change in particle fraction as a function time, showing the distribution of particle disappearance events for each beam voltage.

**Table S1.** Constants and reference parameters used for plots of the charging model

| | parameter | value |
|---|---|---|
| Particle Radius | $r$ | 150 nm |
| Initial particle-IL contact angle | $\theta_0$ | 20°[13] |
| $EMIM^+$ $MeSO_4^-$ surface tension | $\gamma_{L-V}$ | 47 mN/m [14] |
| $EMIM^+$ $MeSO_4^-$ dielectric constant | $\epsilon_R$ | 35[15] |
| $EMIM^+$ $MeSO_4^-$ Debye length | $\lambda_D$ | 3 Å |
| Temperature | $T$ | 298 K |
| Vacuum permittivity | $\epsilon_0$ | 8.854 x $10^{-12}$ F/m |
| Boltzmann's constant | $k_B$ | 8.617 x $10^{-5}$ eV/K |

**Table S2.** Calculated fit parameters for the particle fraction plots in Figures 6D and S10.

| Beam Voltage | $t_s(s)$ | $k(s^{-1})$ |
|---|---|---|
| 2 kV | 93.2 | 0.282 |
| 3 kV | 153.4 | 0.285 |
| 4 kV | 210.9 | 0.300 |
| 5 kV | 265.5 | 0.342 |

## Supplementary Movie Caption

**Movie S1**: Movie of the colloidal monolayer dynamics when exposed to a scanning, focused electron beam, showing clockwise starting in the upper left: the in-lens detector image, grain boundary particles, the bond order parameter magnitude ($|\Psi_{6,j}|$), the bond order parameter phase ($\theta_j$), the change in the bond order parameter ($\Delta|\Psi_{6,j}|$), and the single particle Lindemann parameter ($LP_j$).

## References


1. V. M. Bedanov, G. V. Gadiyak, and Y. E. Lozovik, "On a modified Lindemann-like criterion for 2D melting," Phys. Lett. A **109**, 289–291 (1985).
2. K. Zahn, R. Lenke, and G. Maret, "Two-Stage Melting of Paramagnetic Colloidal Crystals in Two Dimensions," Phys. Rev. Lett. **82**, 2721–2724 (1999).
3. Y. Peng, F. Wang, Z. Wang, A. M. Alsayed, Z. Zhang, A. G. Yodh, and Y. Han, "Two-step nucleation mechanism in solid–solid phase transitions," Nat. Mater. **14**, 101–108 (2015). Number: 1 Publisher: Nature Publishing Group.
4. Y. Peng, W. Li, F. Wang, T. Still, A. G. Yodh, and Y. Han, "Diffusive and martensitic nucleation kinetics in solid-solid transitions of colloidal crystals," Nat. Commun. **8**, 1–12 (2017). Number: 1 Publisher: Nature Publishing Group.
5. P. Dillman, M. Georg, and P. Keim, "Comparison of 2D melting criteria in a colloidal system," J. Physics: Condens. Matter **24** (2012).
6. C. P. Kelleher, R. E. Guerra, A. D. Hollingsworth, and P. M. Chaikin, "Phase behavior of charged colloids at a fluid interface," Phys. Rev. E **95**, 022602 (2017). Publisher: American Physical Society.

7. J. D. Weeks, D. Chandler, and H. C. Andersen, "Role of Repulsive Forces in Determining the Equilibrium Structure of Simple Liquids," J. Chem. Phys. **54**, 5237–5247 (1971).
8. S. Millefiorini, A. H. Tkaczyk, R. Sedev, J. Efthimiadis, and J. Ralston, "Electrowetting of Ionic Liquids," J. Am. Chem. Soc. **128**, 3098–3101 (2006).
9. H. Horiuchi, A. Nikolov, and D. T. Wasan, "Calculation of the surface potential and surface charge density by measurement of the three-phase contact angle," J. Colloid Interface Sci. **385**, 218–224 (2012).
10. H. Weingärtner, "Understanding Ionic Liquids at the Molecular Level: Facts, Problems, and Controversies," Angew. Chem. Int. **47**, 654–670 (2008). _eprint: https://onlinelibrary.wiley.com/doi/pdf/10.1002/anie.200604951.
11. S. Perkin, L. Crowhurst, H. Niedermeyer, T. Welton, A. M. Smith, and N. N. Gosvami, "Self-assembly in the electrical double layer of ionic liquids," Chem. Commun. **47**, 6572 (2011).
12. M. A. Gebbie, A. M. Smith, H. A. Dobbs, A. A. Lee, G. G. Warr, X. Banquy, M. Valtiner, M. W. Rutland, J. N. Israelachvili, S. Perkin, and R. Atkin, "Long range electrostatic forces in ionic liquids," Chem. Commun. **53**, 1214–1224 (2017).
13. P. Y. Kim, Y. Gao, Y. Chai, P. D. Ashby, A. E. Ribbe, D. A. Hoagland, and T. P. Russell, "Assessing Pair Interaction Potentials of Nanoparticles on Liquid Interfaces," ACS Nano **13**, 3075–3082 (2019).
14. M. Tariq, M. G. Freire, B. Saramago, J. A. P. Coutinho, J. N. C. Lopes, and L. P. N. Rebelo, "Surface tension of ionic liquids and ionic liquid solutions," Chem. Soc. Rev. **41**, 829–868 (2012). Publisher: The Royal Society of Chemistry.
15. M.-M. Huang, Y. Jiang, P. Sasisanker, G. W. Driver, and H. Weingärtner, "Static Relative Dielectric Permittivities of Ionic Liquids at 25 °C," J. Chem. & Eng. Data **56**, 1494–1499 (2011). Publisher: American Chemical Society.
